# Supplementary material for: HiWave: Training-Free High-Resolution Image Generation via Wavelet-Based Diffusion Sampling
Source: arXiv:2506.20452 source file (2025-06-25)
Supplement: Supplementary file 1 [file appendix_copy.tex]

\section{Quantitative Evaluation}

\begin{table*}[htp]
\caption{Quantitative comparison of high-resolution image generation methods. Results based on 1000 random samples from the LAION/LAION2B-en-aesthetic dataset. "Ours+CC" includes color correction to address saturation reduction.}
\begin{tabular}{c|l|c|c|c|c|c|c}
\hline
\textbf{Resolution} & \textbf{Model} & \textbf{FID}$\downarrow$ & \textbf{KID}$\downarrow$ & \textbf{IS}$\uparrow$ & \textbf{CLIP}$\uparrow$ & \textbf{LPIPS}$\downarrow$ & 
\textbf{ HPS-v2 }$\uparrow$\\
\hline
$1024^2$ & SDXL & \textbf{61.78}  & \textbf{0.0020} & 18.6651 & 33.2183 & \textbf{0.7779} & \textbf{0.2639} \\
\hline
\multirow{3}{*}{$2048^2$} & HiWave & 63.3460   & 0.0027 & \textbf{19.4784} & 33.2568 & 0.7784  & 0.2620 \\
 & Pixelsmith &  62.3054   & 0.002197 & 19.1222 & 33.1550 & 0.7808 & 0.2598 \\
  & HiDiffusion & 65.9073   & 0.002895 & 17.7217 & 31.9566 & 0.7834 & 0.2432 \\
  & SDXL & 92.4854   & 0.010774 & 14.0658 & 31.3733 & 0.7828 & 0.2274\\
\hline
\multirow{3}{*}{$4096^2$} & HiWave & 64.7265    & 0.003241 & 18.7743 & \textbf{33.2729} & 0.7831 & 0.2585\\
& HiWave+CC & 64.7538    & 0.003129 & 18.8701 & 33.2294 & 0.8139 &  0.2610\\
 & Pixelsmith & 62.5542  & 0.002373 & 19.4302 &  33.1504 & 0.8039 & 0.2598 \\
& HiDiffusion &  93.4473  &  0.014934  & 14.6960  & 28.2296  & 0.7996 & 0.1821 \\
\hline
\end{tabular}
\label{tab:metrics}
\end{table*}

Table \ref{tab:metrics} provides a quantitative comparison using several standard metrics common in generative image synthesis evaluation. While these metrics offer valuable insights into model performance, it is crucial to acknowledge their limitations, particularly when evaluating the high-resolution outputs (e.g., 2048x2048 and 4096x4096) produced by methods like HiWave.
A significant factor is that many of these metrics rely on underlying neural network architectures that operate on fixed, lower-resolution inputs. Consequently, evaluating our high-resolution generated images necessitates substantial downsampling, which may not fully capture the improvements in fine-grained details, textures, and overall fidelity that high-resolution synthesis aims to achieve.

Specifically:

\textbf{FID (Fréchet Inception Distance)} \cite{heusel2017gans} and KID (Kernel Inception Distance) \cite{binkowski2018demystifying}: These widely used metrics compare feature representations extracted by the Inception V3 network \cite{szegedy2016rethinking}. Inception V3 requires input images to be resized to 299x299 pixels. Downsampling from 4096x4096 to 299x299 inevitably leads to a loss of high-frequency information.

\textbf{IS (Inception Score)} \cite{salimans2016improved}: Similarly, the Inception Score relies on the Inception V3 network and thus requires images to be resized to 299x299 pixels. While indicative of image quality and diversity at that scale, it doesn’t assess details only visible at higher resolutions.

\textbf{CLIP Score}: This metric evaluates the semantic alignment between the generated image and the input text prompt using embeddings from the CLIP model \cite{radford2021learning}. Commonly used CLIP vision encoders, such as ViT-L/14 or ViT-B/32, process images at a resolution of 224x224 pixels. This significant downsampling primarily captures semantic content rather than high-resolution fidelity.

\textbf{LPIPS (Learned Perceptual Image Patch Similarity)} \cite{zhang2018unreasonable}: LPIPS measures perceptual similarity using features from networks like AlexNet or VGG. While designed to correlate well with human perception, standard implementations often process images resized to resolutions like 256x256 pixels, limiting their ability to assess fine details present only at much higher resolutions.

\textbf{HPS-v2 (Human Preference Score v2)} \cite{wu2023human}: While HPS v2 addresses limitations of earlier metrics by aligning better with human aesthetic judgment, it still relies on the CLIP ViT-H/14 architecture \cite{radford2021learning}, which processes images at 224x224 resolution. Therefore, evaluating our 4096x4096 outputs requires the same significant downsampling as the CLIP score, potentially losing some of the fine details our method aims to preserve.

\section{Duplication Artifact Analysis}

\begin{figure}[htp]
  \centering
  \includegraphics[width=0.45\textwidth]{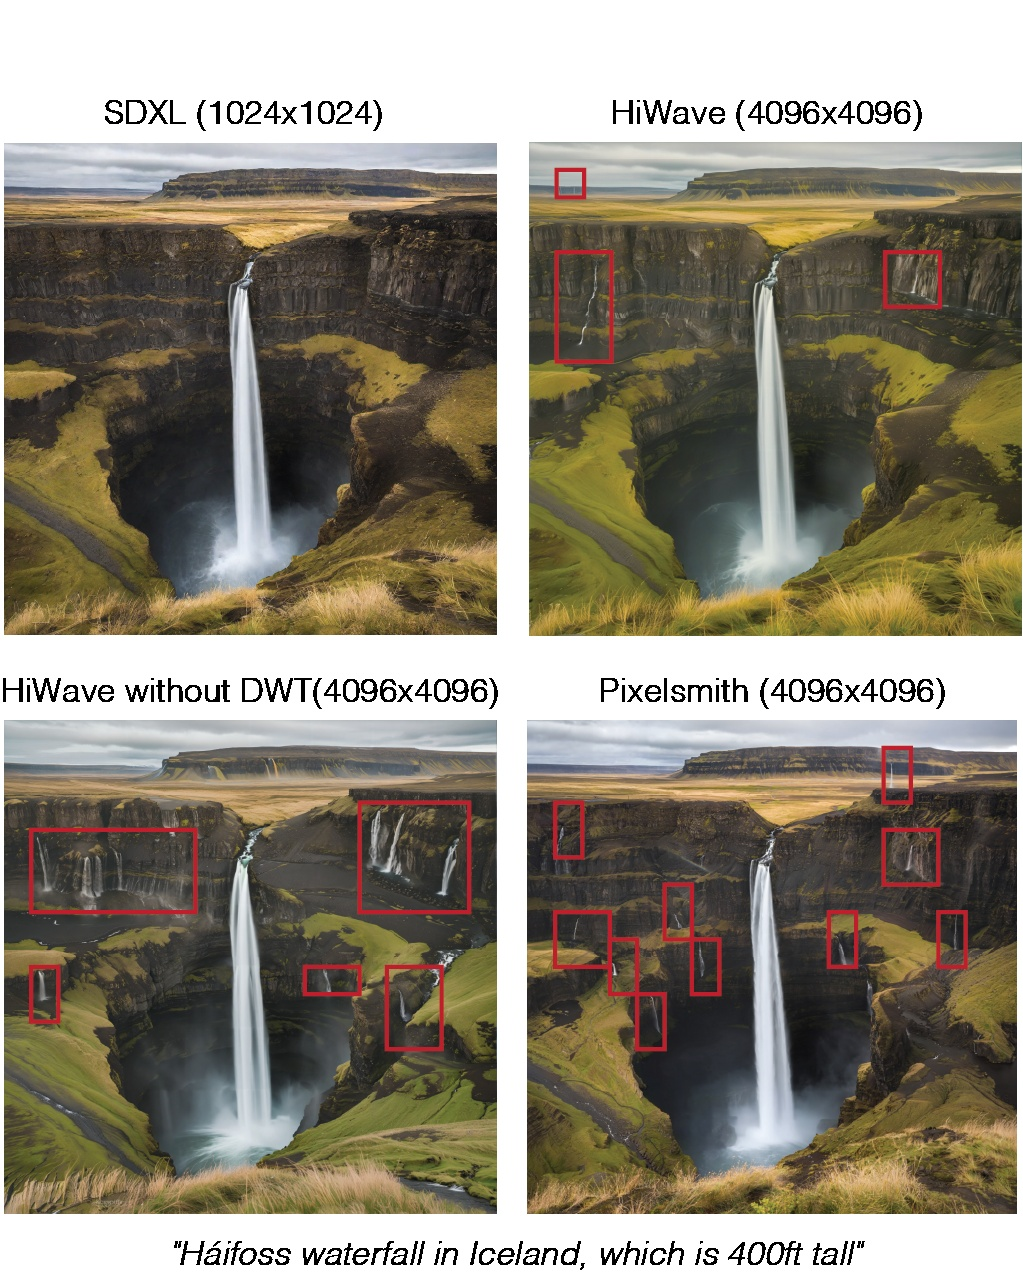}
  \caption{Comparison of duplication artifacts in high-resolution (4096$\times$4096) generation of Háifoss waterfall. Red boxes highlight duplicated elements. Top left: SDXL baseline (1024$\times$1024) with no duplications. Top right: Our HiWave method with minimal duplications. Bottom left: Our method without DWT guidance shows several duplicate waterfalls. Bottom right: Pixelsmith exhibits extensive duplication artifacts throughout the scene.}
  \label{fig:duplication_comparison}
\end{figure}

Standard quantitative metrics often fail to capture duplication artifacts, one of the most perceptually significant issues in path based methods. Figure \ref{fig:duplication_comparison} provides a direct visual comparison of how different methods handle this challenge using a waterfall scene, which is particularly prone to duplication due to its repetitive natural features.

The SDXL baseline correctly generates a single waterfall at its native resolution, while our HiWave method at 4096$\times$4096 resolution maintains this structural integrity with only minimal duplications in background regions. In contrast, our ablation without DWT guidance generates several noticeable duplicate waterfalls, demonstrating the effectiveness of our frequency-aware approach. Pixelsmith produces numerous duplications throughout the scene, significantly compromising the image's realism.

This visualization confirms that while no patch-based method completely eliminates duplications in challenging scenarios, our DWT-guided approach substantially reduces these artifacts compared to the current state-of-the-art.

\section{Computational Performance}

\begin{table}[t]
  \centering
  \caption{Inference time comparison (seconds) for different high-resolution image generation methods. Comparative data from Pixelsmith \cite{tragakis2024one} with our method's measurements added.}
  \begin{tabular}{lcc}
    \hline
    \textbf{Model} & \textbf{2048²} & \textbf{4096²} \\
    \hline
    SDXL & 71 & 515 \\
    ScaleCrafter \cite{he2023scalecrafter} & 80 & 1257 \\
    DemoFusion \cite{du2024demofusion} & 219 & 1632 \\
    HiDiffusion \cite{zhang2023hidiffusion} & 50 & 255 \\
    FouriScale \cite{huang2024fouriscale} & 162 & OOM* \\
    AccDiffusion \cite{lin2024accdiffusion} & 231 & 1710 \\
    Pixelsmith \cite{tragakis2024one} & 130 & 549 \\
    HiWave & 238 & 1557 \\
    \hline
  \end{tabular}
  \label{tab:inference_time}
  \\ \small{*All measurements except for ours are from \cite{tragakis2024one}. Measured on NVIDIA RTX 3090, OOM: Out of memory on RTX 3090.}
\end{table}


Table \ref{tab:inference_time} presents the inference times for various high-resolution generation methods. It's important to note that the relatively higher inference time of our method compared to Pixelsmith is primarily due to methodological differences rather than the DWT computation overhead. Our approach performs a complete 50-step diffusion process for maximum quality, while Pixelsmith utilizes a reduced 20-step pipeline that sacrifices some quality for speed. When accounting for this difference in sampling steps, our method's performance is in line with other patch-based approaches. This design decision prioritizes image quality over raw computational efficiency, which we consider a reasonable trade-off given the significant improvements in our qualitative results.

\section{Structural Improvements Over Base Generation}

In \ref{fig:improvs_SDXL}, we compare SDXL base generations with our HiWave upscaling method across a range of challenging content types. The examples include cropped regions that represent 1/5 the width of the original images (SDXL at 1024$\times$1024, HiWave at 4096$\times$4096). HiWave consistently enhances facial definition (Rows 1–3) and produces sharper character renderings (Row 4), while faithfully preserving the global composition and visual style of the original generations.
%
\begin{figure}[htp]
  \centering
  \includegraphics[width=0.9\linewidth]{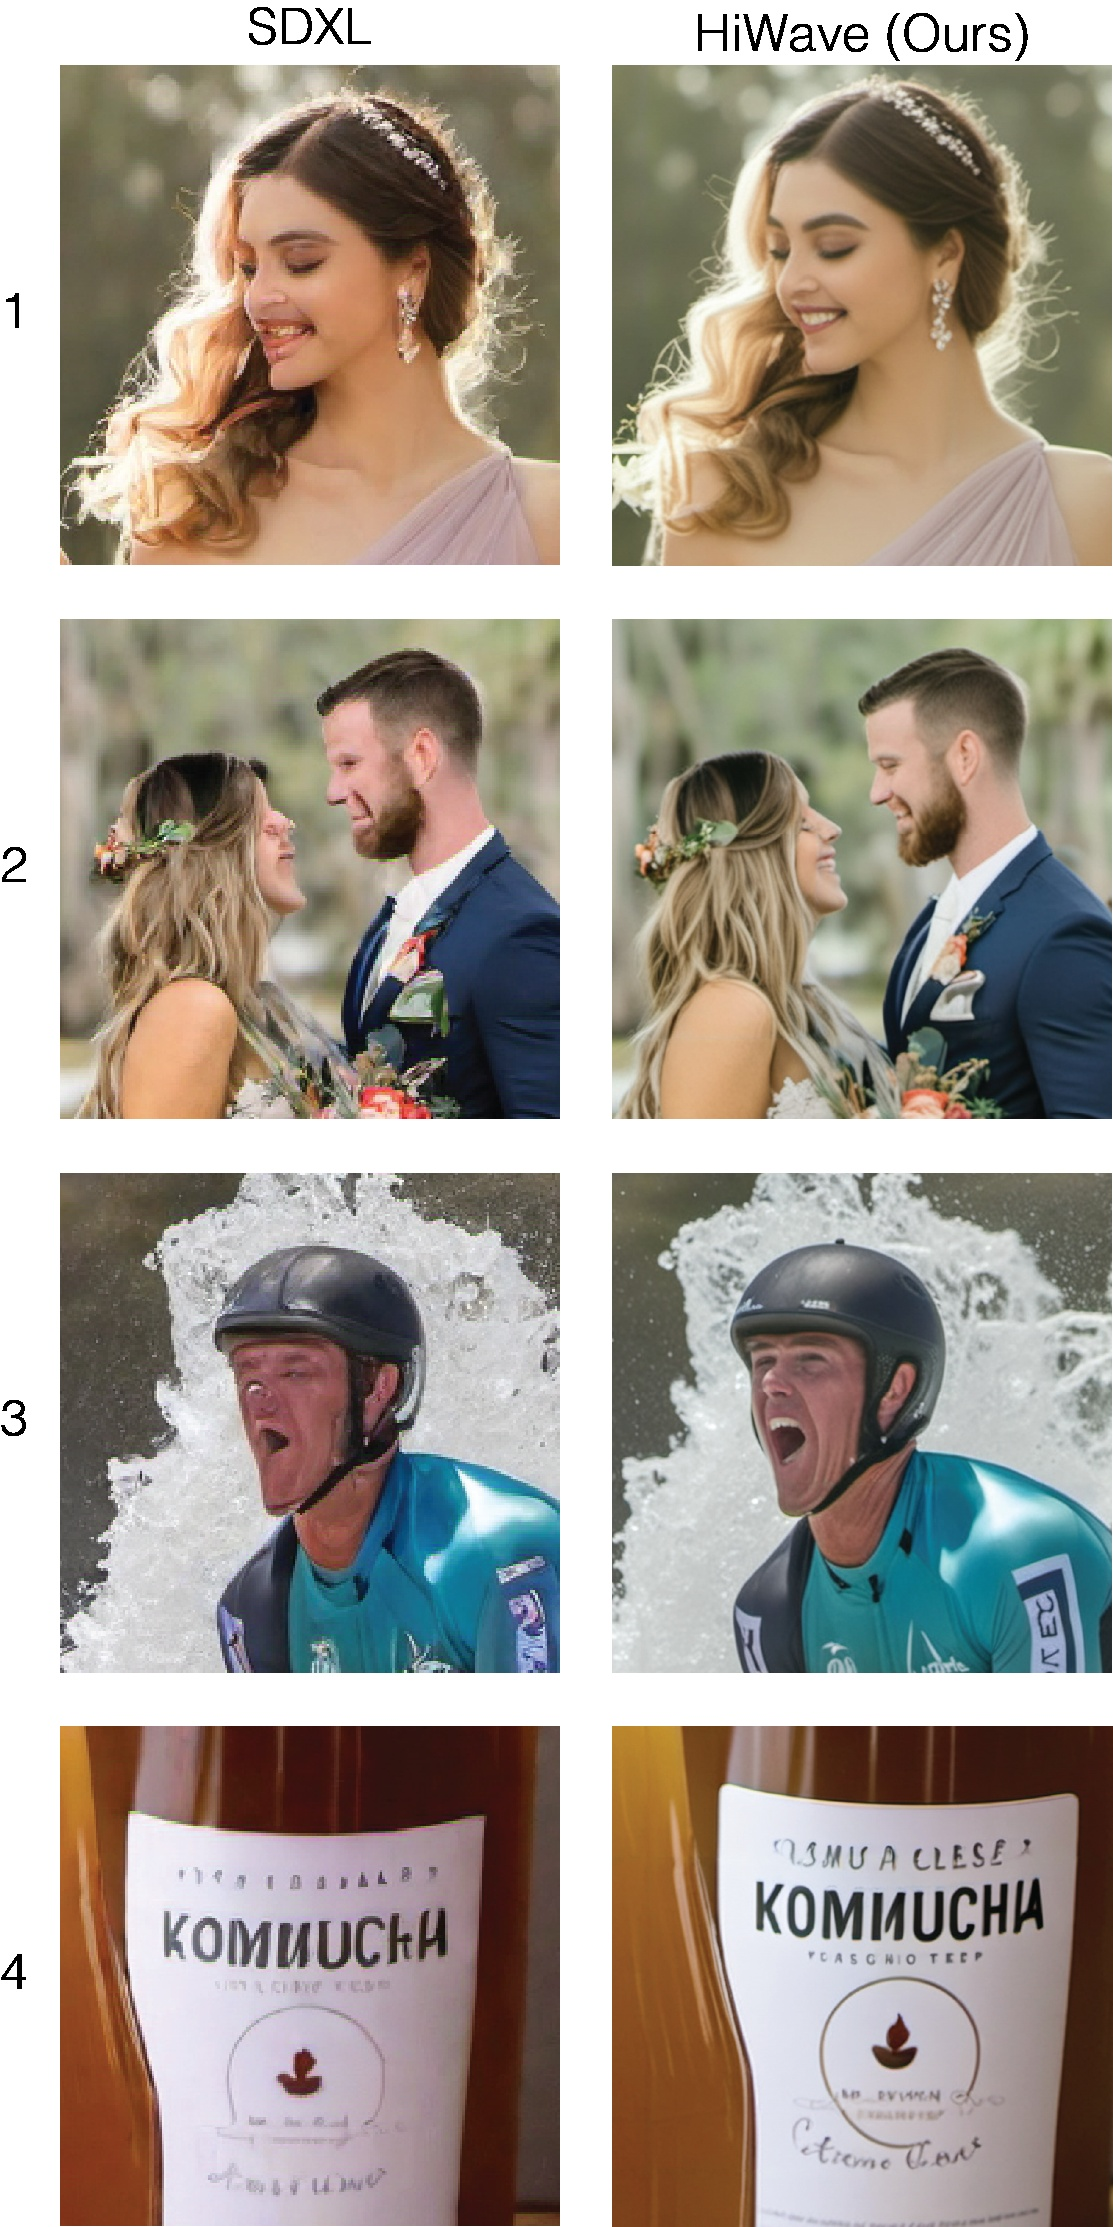}
  \caption{Comparison between SDXL base generations and our HiWave upscaling method across various challenging content types. The shown crops are 1/5 the length of the original images (SDXL: 1024$\times$1024, HiWave: 4096$\times$4096). Our approach enhances facial definition (Rows 1–3) and renders sharper characters (Row 4), while preserving the global composition and visual style.}
  \label{fig:improvs_SDXL}
\end{figure}


\section{Frequency Band Guidance Configurations}
In \autoref{fig:bands_configurations}, we compare different configurations of our frequency guidance strategy. The top-left image shows the SDXL base generation at 1024$\times$1024 resolution, while the top-right displays the result of our full HiWave method with DWT-based guidance at 4096$\times$4096. To analyze the role of frequency-specific control, the bottom-left variant applies guidance only to low-frequency bands---that is the opposite of HiWave---while the bottom-right replaces our DWT approach with conventional classifier-free guidance (CFG) applied uniformly across all frequency components. Both the low-frequency-only and the CFG-only variants introduce noticeable duplication artifacts, indicating weakened structural control, whereas HiWave preserves the global composition of the original SDXL image while enriching fine details.


\begin{figure}[htp]
  \centering
  \includegraphics[width=0.9\linewidth]{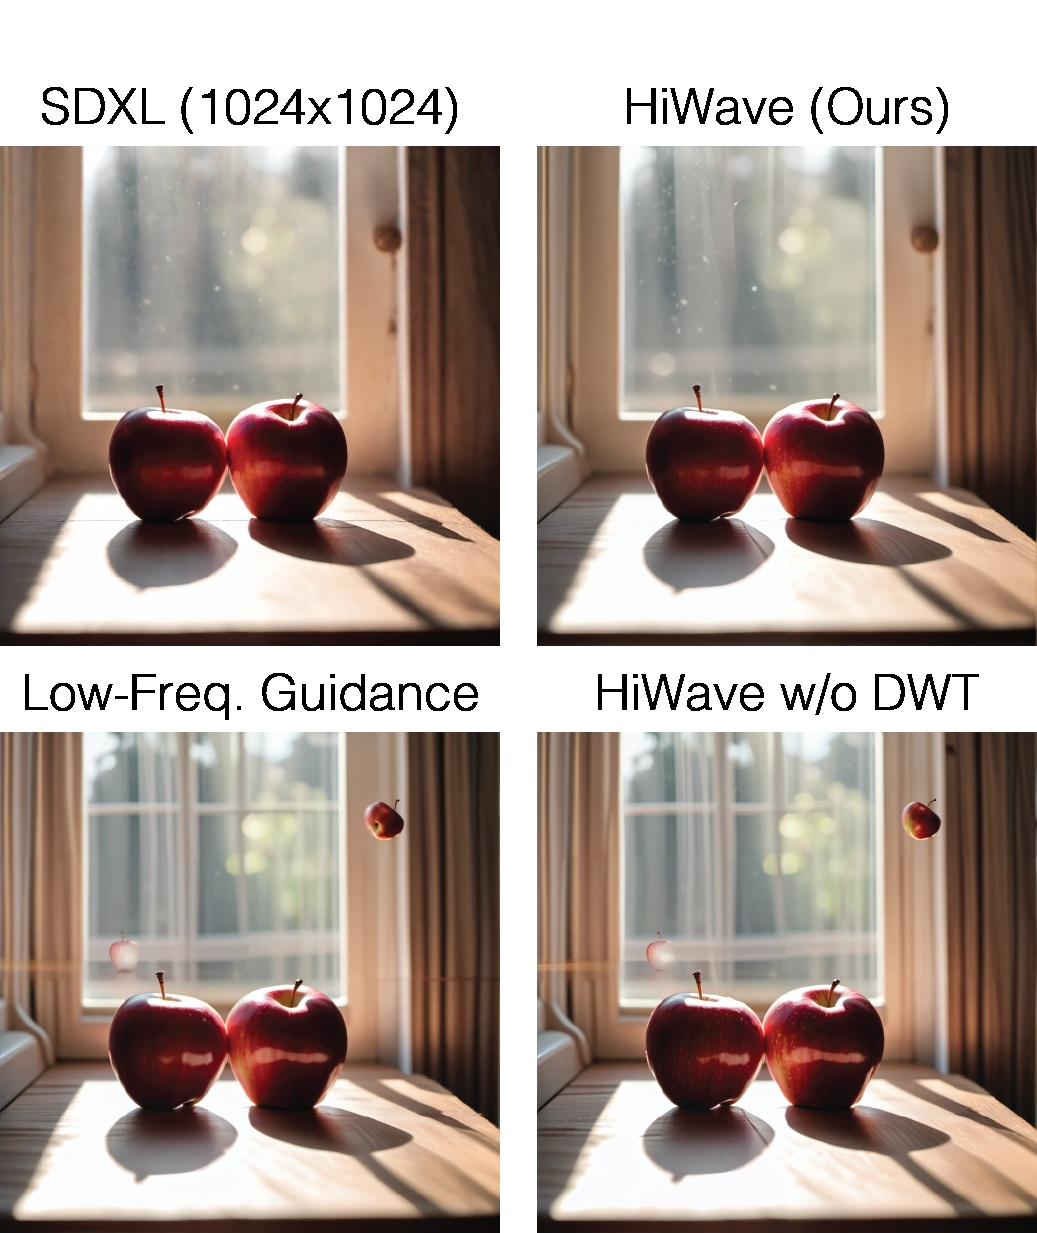}
  \caption{Comparison of different configurations of frequency guidance. The top-left shows the SDXL base image at 1024$\times$1024 resolution. The top-right is our full HiWave method with DWT-based guidance at 4096$\times$4096. The bottom-left applies guidance only to the low-frequency bands (i.e., the opposite of our method). The bottom-right replaces our DWT strategy with conventional classifier-free guidance (CFG) applied uniformly.}
  \label{fig:bands_configurations}
\end{figure}

\section{Importance of DDIM Inversion}
To illustrate the effect of omitting DDIM inversion in HiWave, in \autoref{fig:noDDIM}, we compare results with and without this component. On the left, HiWave is applied without DDIM inversion, while the right shows the output of the full HiWave method. Without DDIM inversion, patch-wise generation becomes independent and uncoordinated, leading to visible seams, geometric inconsistencies, and color mismatches across patch boundaries. In contrast, the full HiWave method maintains spatial coherence across the entire image.

\begin{figure}[htp]
  \centering
  \includegraphics[width=0.9\linewidth]{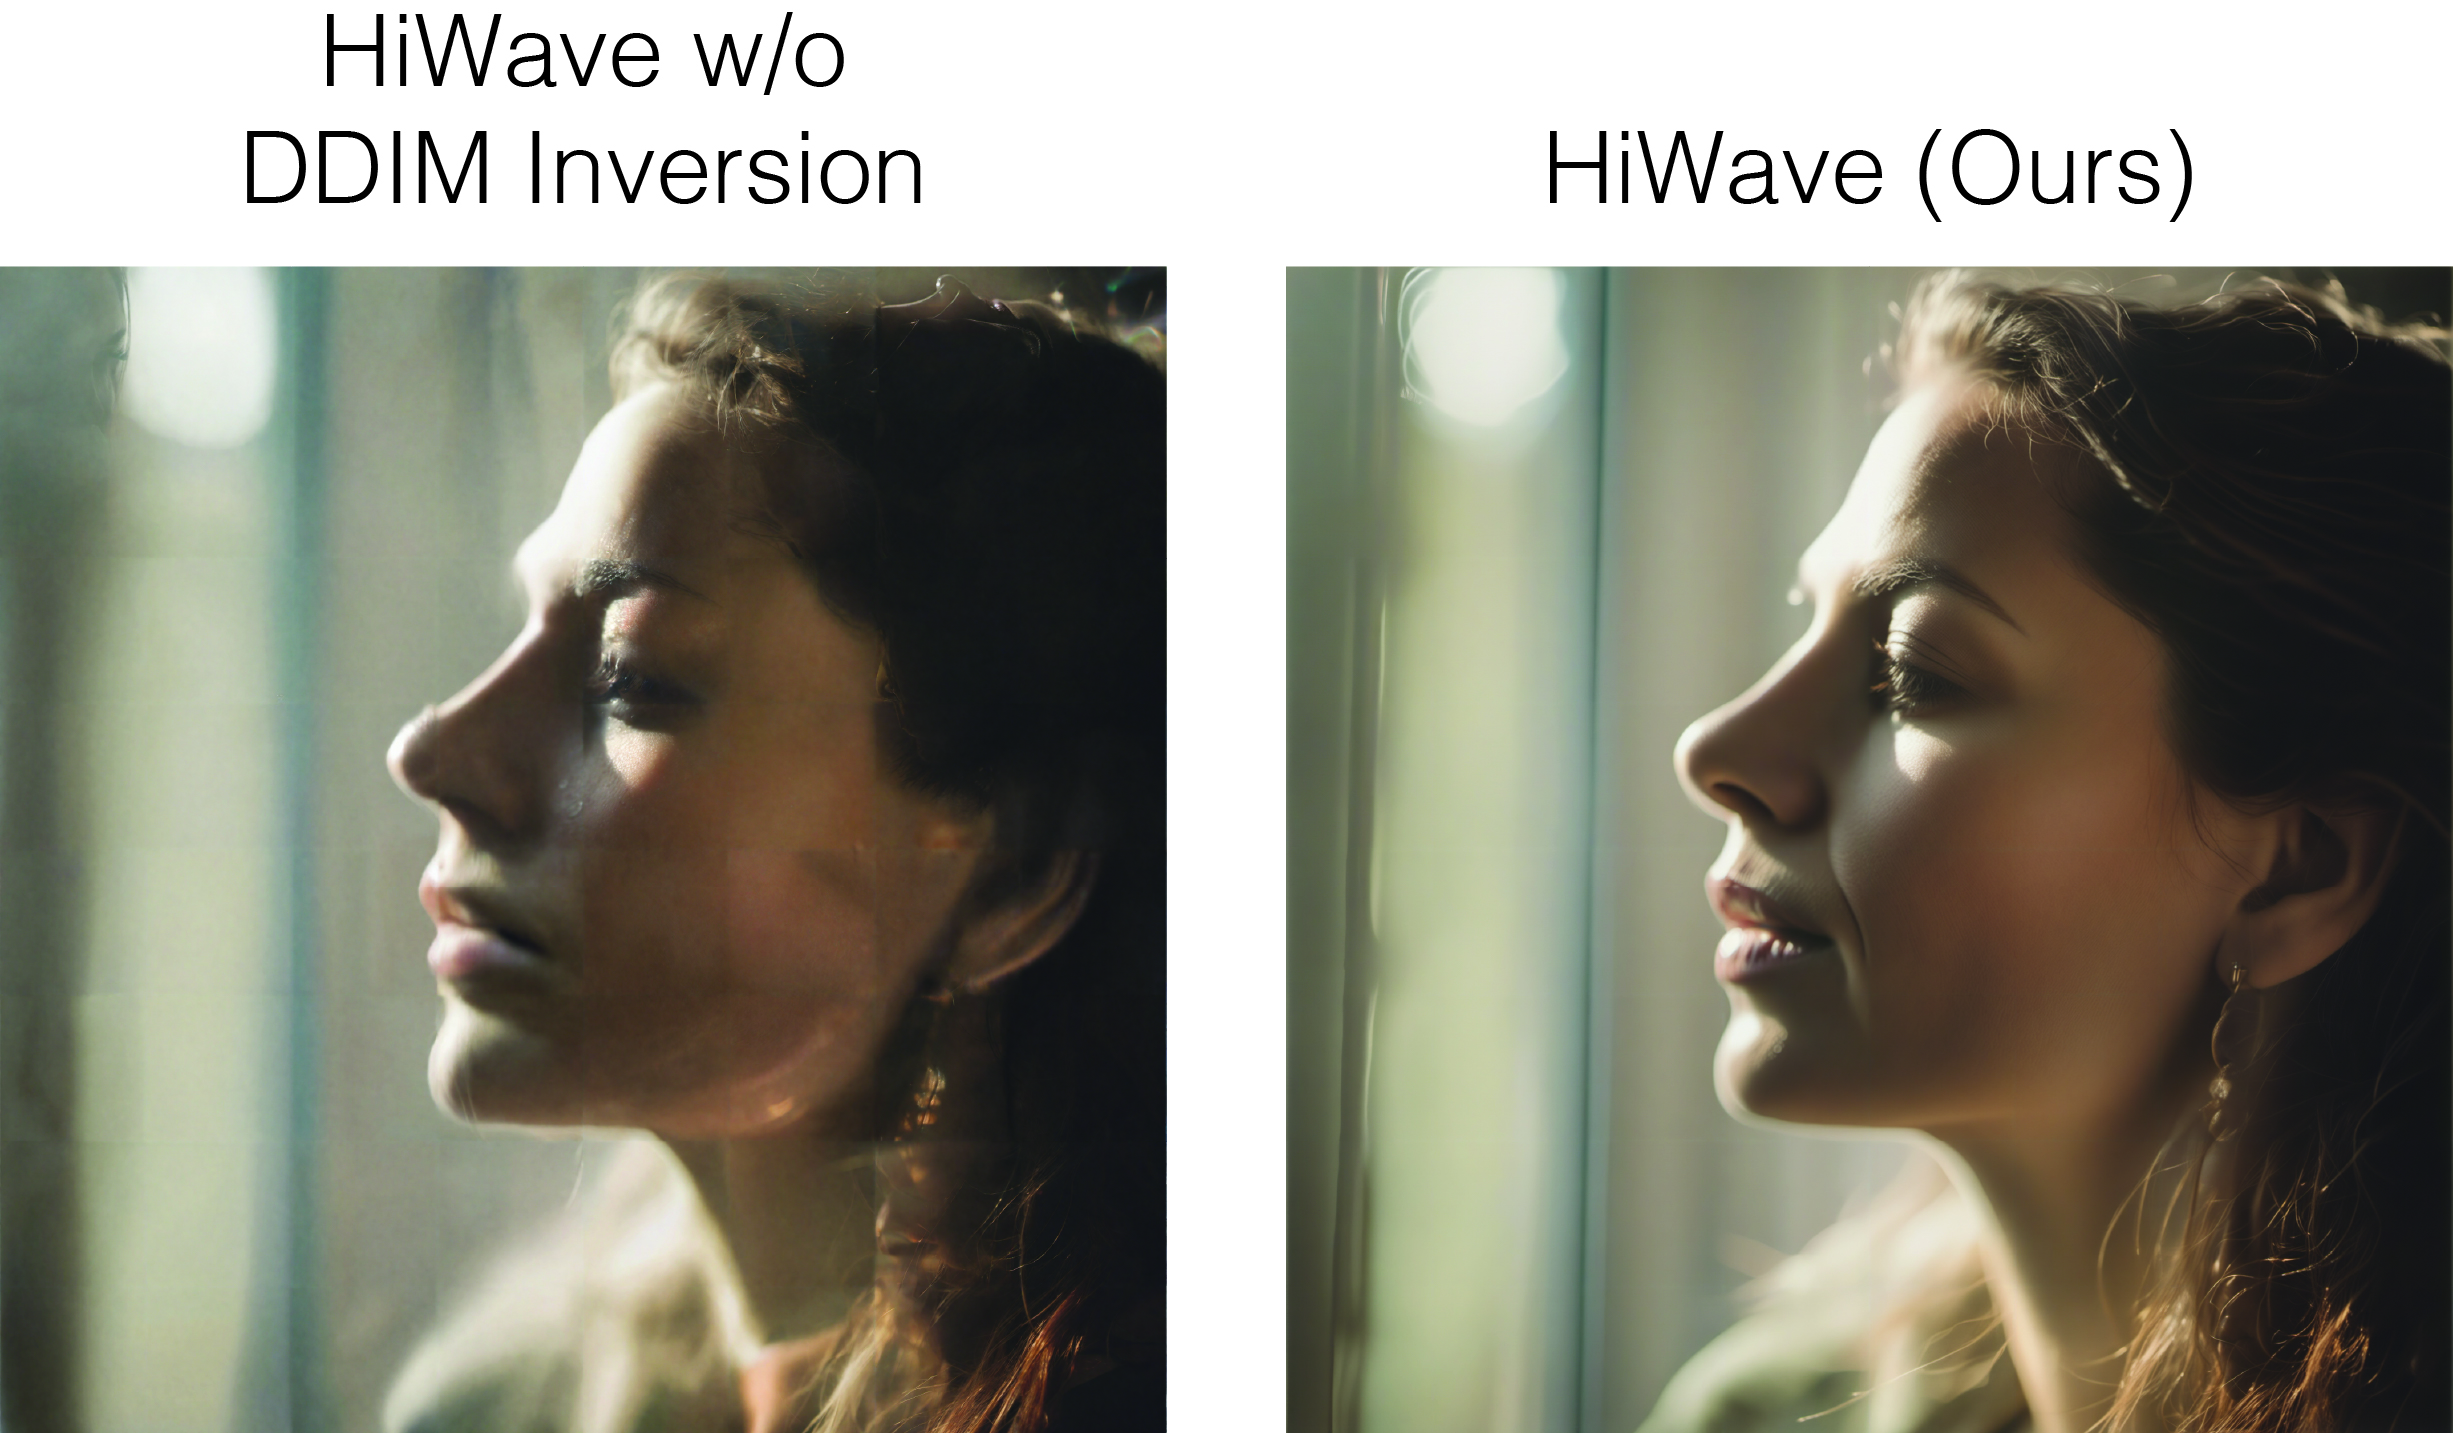}
  \caption{Effect of omitting DDIM inversion in HiWave. Left: HiWave without DDIM inversion. Right: Full HiWave method. Without DDIM inversion, patch-wise generation becomes independent, resulting in visible seams, inconsistent geometry, and color mismatches across patches.}
  \label{fig:noDDIM}
\end{figure}

\section{One-Shot vs Multi-Step Generation}

\begin{figure}[htp]
  \centering
  \includegraphics[width=0.9\linewidth]{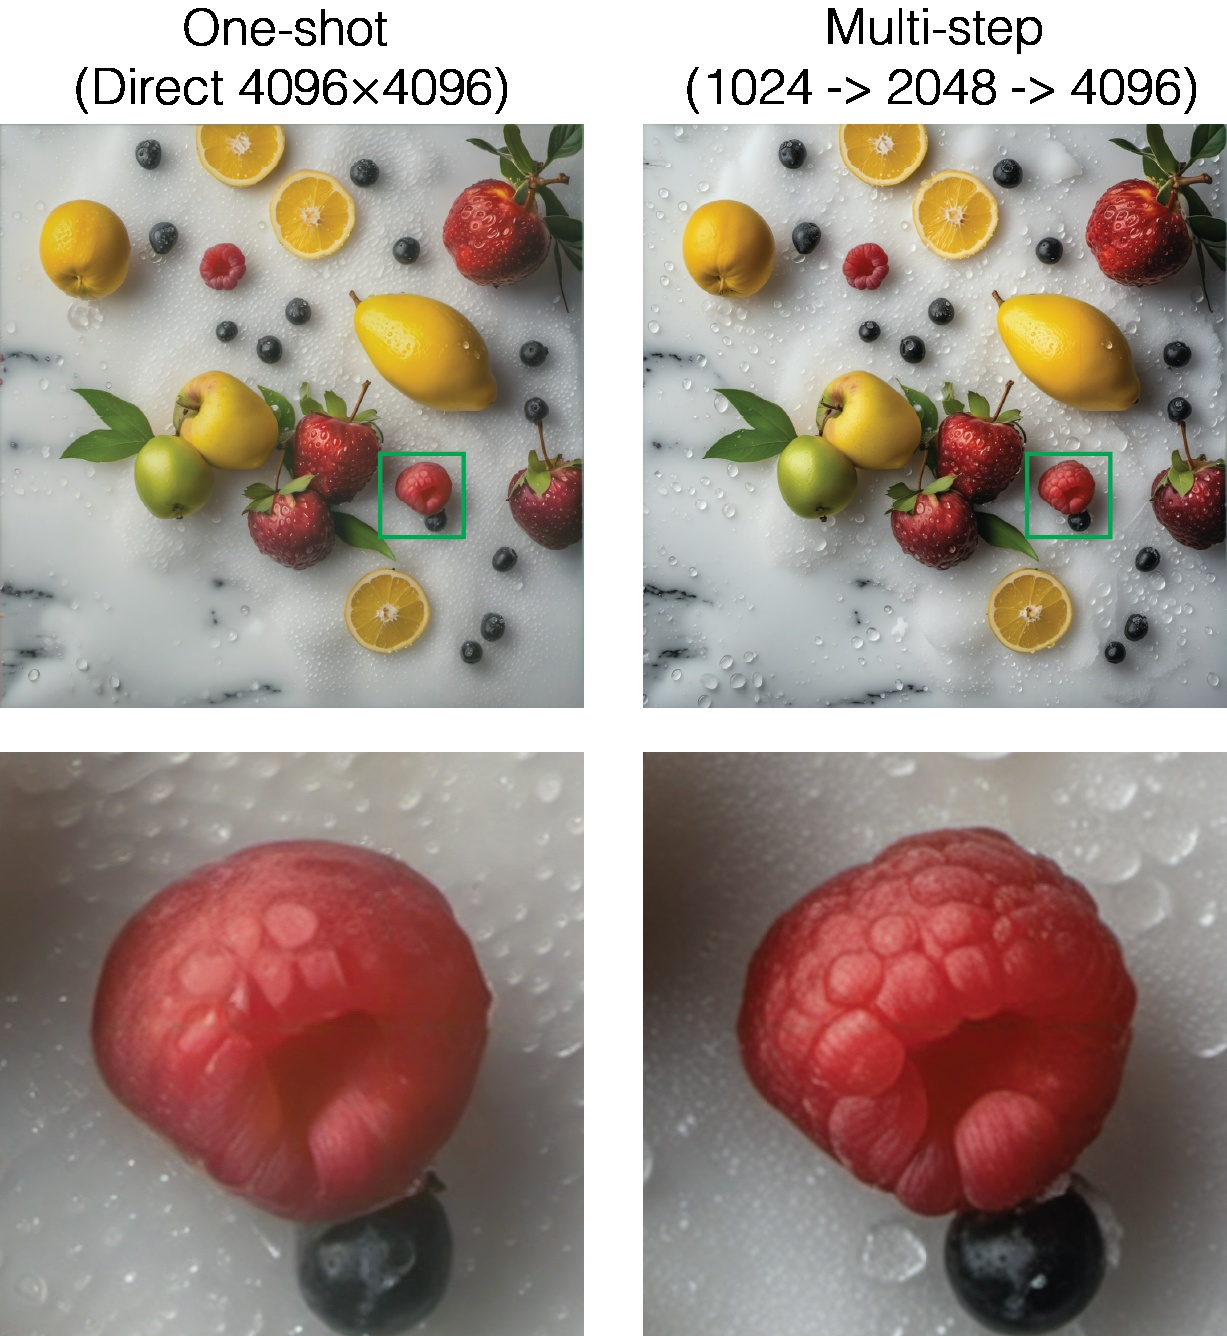}
  \caption{}
  \label{fig:oneShotvsMulti}
\end{figure}



% \input{scripts/table_human_eval}
